# Supplementary material for: Edge-preserving Near-light Photometric Stereo with Neural Surfaces
Source: arXiv:2207.04622 source file (2022-07-11)
Supplement: Supplementary file 1 [file supp_synthetic_comp_normal.tex]

\resizebox{1\textwidth}{!}{
		\large
		\begin{tabular}{@{}c:c@{}@{}c@{}@{}c@{}@{}c@{}@{}c@{}}
			GT shape &QD18~\cite{queau2018led}   &LB20~\cite{logothetis2020cnn} & SM20~\cite{santo2020deep}   &MQ16~\cite{mecca2016single} & Ours  \\
			{\includegraphics[ width=\imgsize\textwidth, trim={65px 65px 65px 65px},clip]{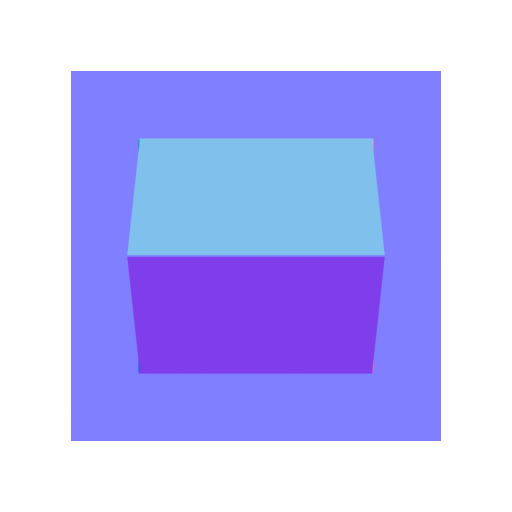}}
			&{\includegraphics[ width=\imgsize\textwidth, trim={65px 65px 65px 65px},clip]{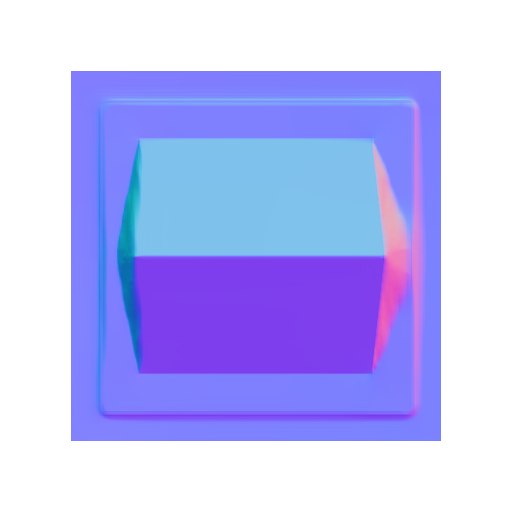}}
			&{\includegraphics[ width=\imgsize\textwidth, trim={65px 65px 65px 65px},clip]{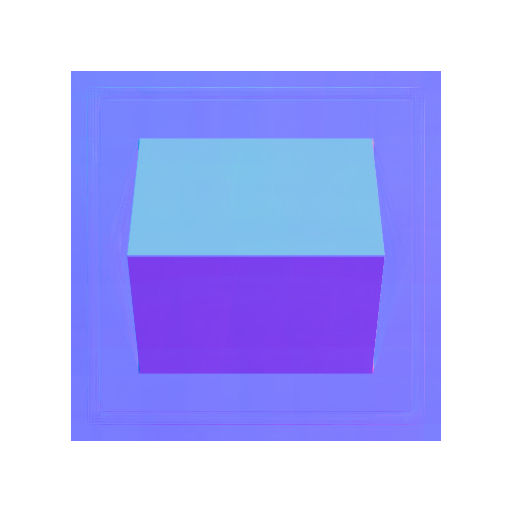}}
			&{\includegraphics[ width=\imgsize\textwidth, trim={65px 65px 65px 65px},clip]{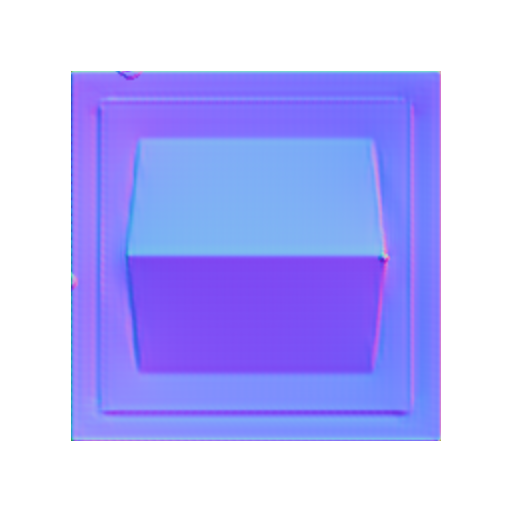}}
			&{\includegraphics[ width=\imgsize\textwidth, trim={65px 65px 65px 65px},clip]{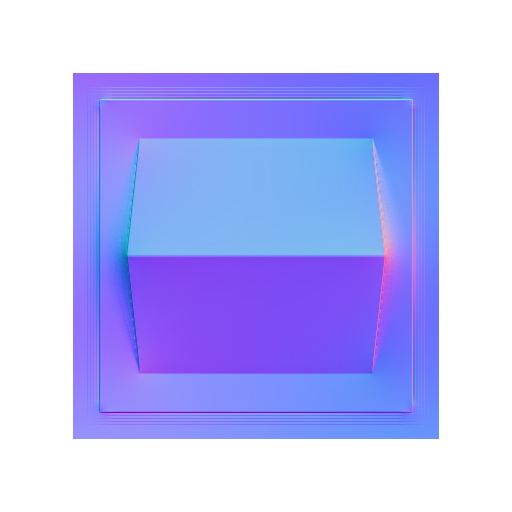}}
			&{\includegraphics[ width=\imgsize\textwidth, trim={65px 65px 65px 65px},clip]{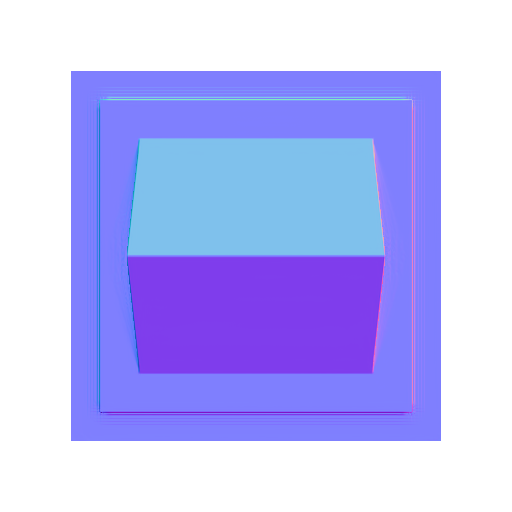}}
			\\
			{\sc Tent} & 5.41  & 2.29  & 9.99  & 10.99  & 1.72  
			\\
			&{\includegraphics[ width=\imgsize\textwidth, trim={65px 65px 65px 65px},clip]{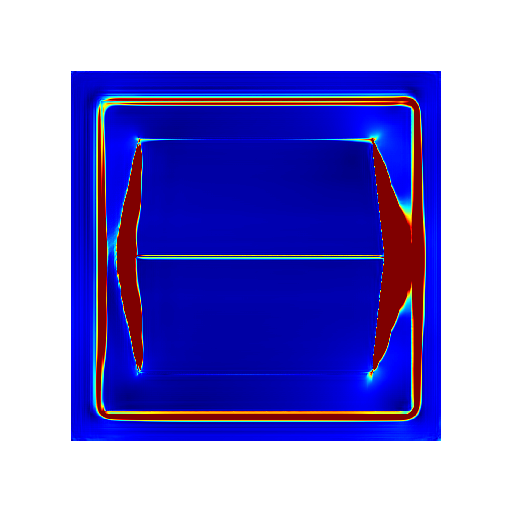}}
			&{\includegraphics[ width=\imgsize\textwidth, trim={65px 65px 65px 65px},clip]{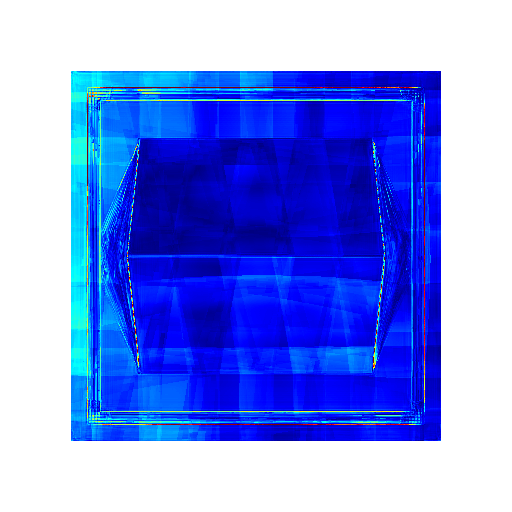}}
			&{\includegraphics[ width=\imgsize\textwidth, trim={65px 65px 65px 65px},clip]{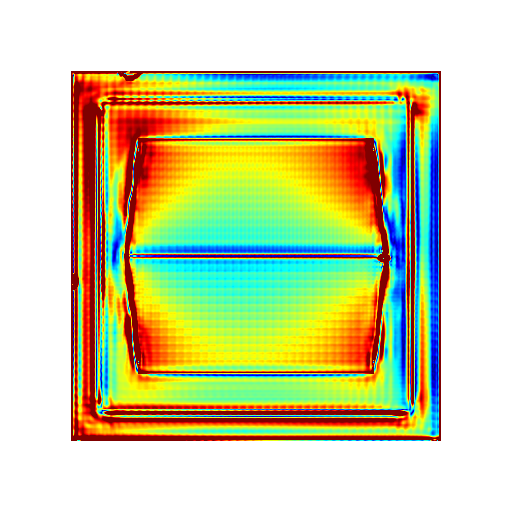}}
			&{\includegraphics[ width=\imgsize\textwidth, trim={65px 65px 65px 65px},clip]{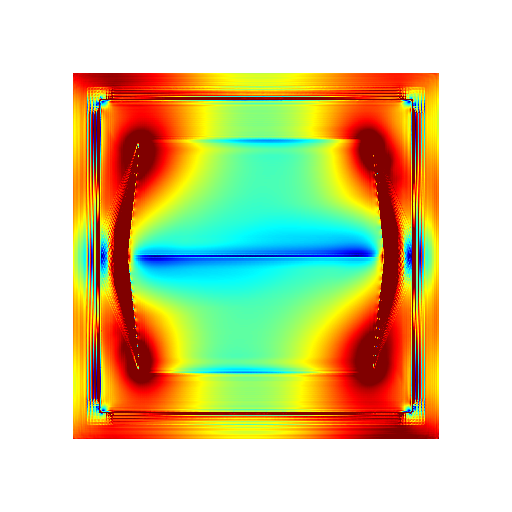}}
			&{\includegraphics[ width=\imgsize\textwidth, trim={65px 65px 65px 65px},clip]{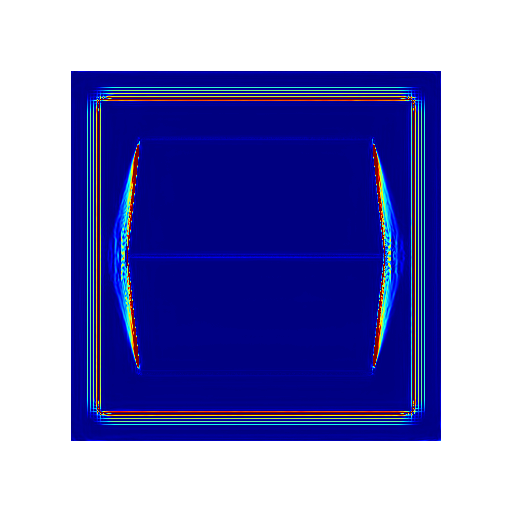}}
			\begin{minipage}{0.02\textwidth} \centering
				\vspace{-5.5em} \makebox[0.5\textwidth]{ $\;\; 15^{\circ}$}\\ \vspace{-0em}
				\makebox[0.5\textwidth]{}\includegraphics[width=0.7\linewidth]{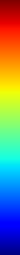} \\ \vspace{-0.4em}
				\makebox[0.5\textwidth]{ $\;\; 0^{\circ}$}\\
			\end{minipage}\\
			{\includegraphics[ width=\imgsize\textwidth, trim={10px 0px 40px 33px},clip]{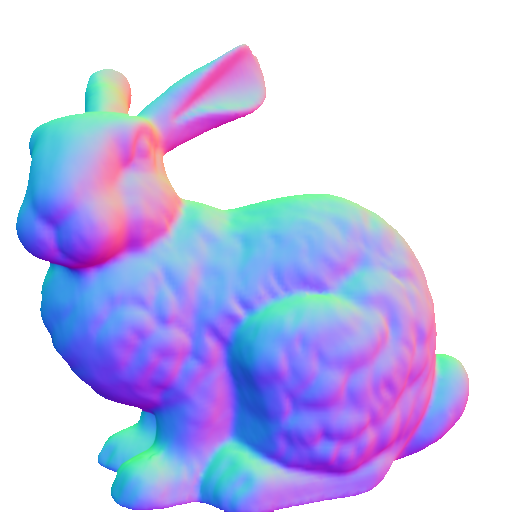}}
			&{\includegraphics[ width=\imgsize\textwidth, trim={10px 0px 40px 33px},clip]{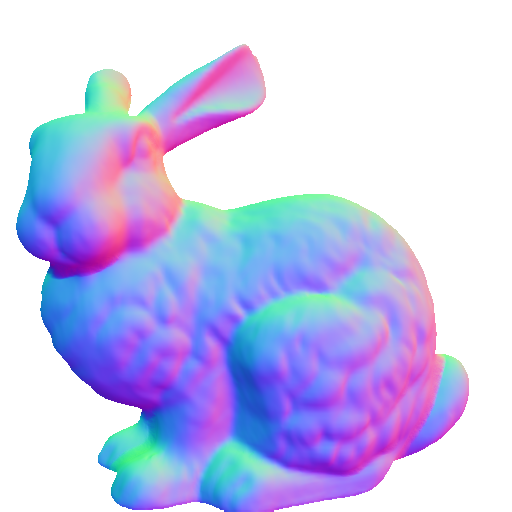}}
			&{\includegraphics[ width=\imgsize\textwidth, trim={10px 0px 40px 33px},clip]{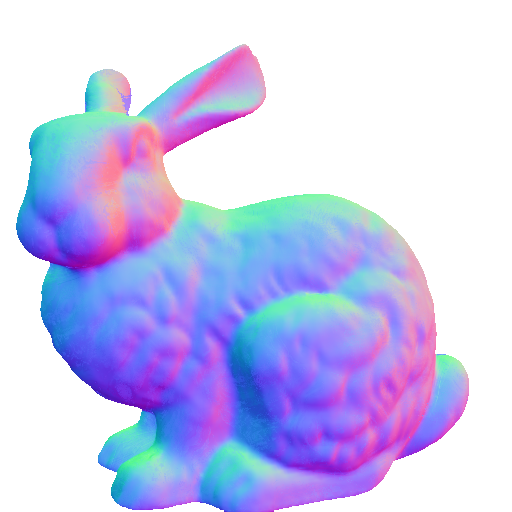}}
			&{\includegraphics[ width=\imgsize\textwidth, trim={10px 0px 40px 33px},clip]{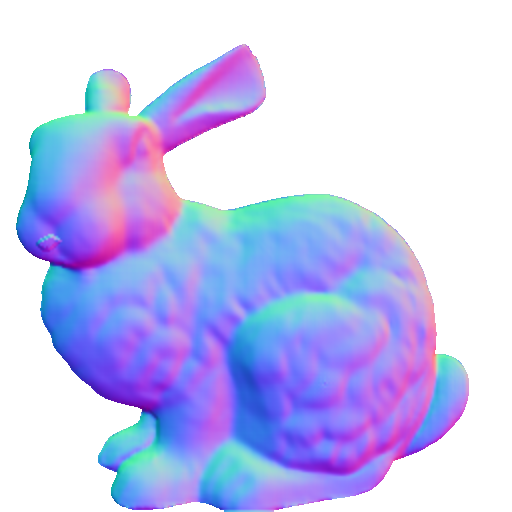}}
			&{\includegraphics[ width=\imgsize\textwidth, trim={10px 0px 40px 33px},clip]{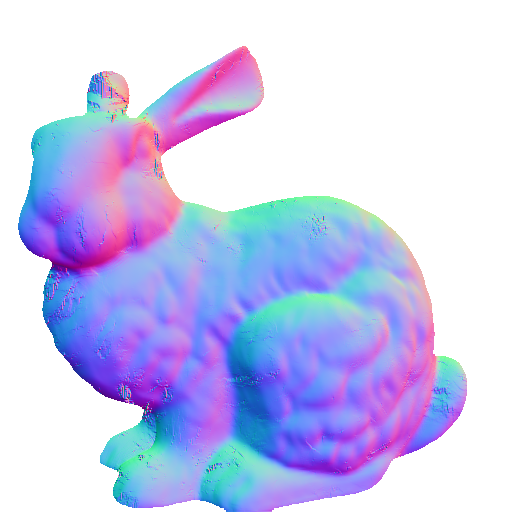}}
			&{\includegraphics[ width=\imgsize\textwidth, trim={10px 0px 40px 33px},clip]{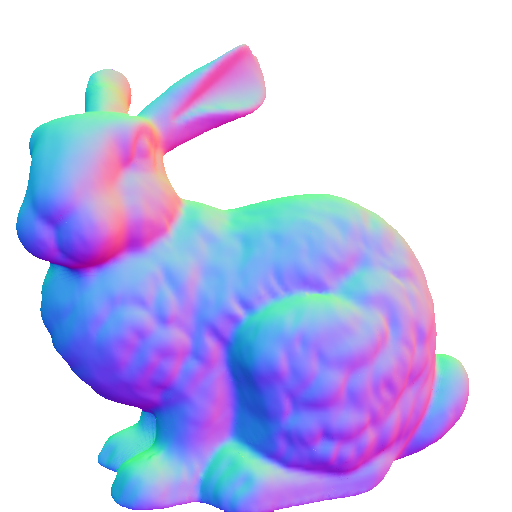}}
			\\
			{\sc Bunny} & 1.66 & 3.94  & 7.43  & 8.54  & 0.33 
			\\
			&{\includegraphics[ width=\imgsize\textwidth, trim={10px 0px 40px 33px},clip]{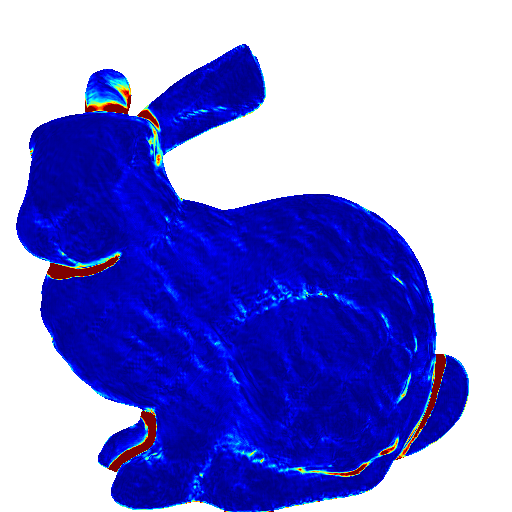}}
			&{\includegraphics[ width=\imgsize\textwidth, trim={10px 0px 40px 33px},clip]{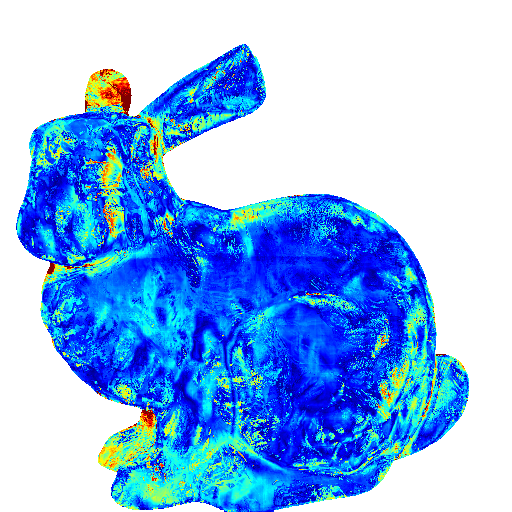}}
			&{\includegraphics[ width=\imgsize\textwidth, trim={10px 0px 40px 33px},clip]{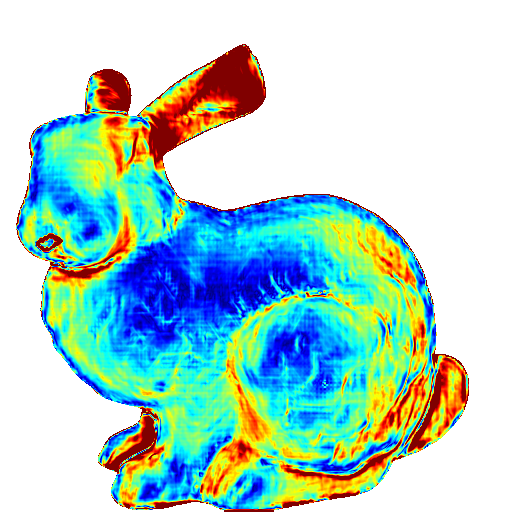}}
			&{\includegraphics[ width=\imgsize\textwidth, trim={10px 0px 40px 33px},clip]{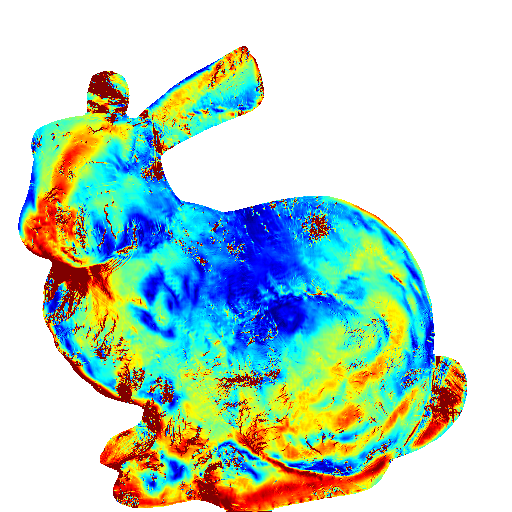}}
			&{\includegraphics[ width=\imgsize\textwidth, trim={10px 0px 40px 33px},clip]{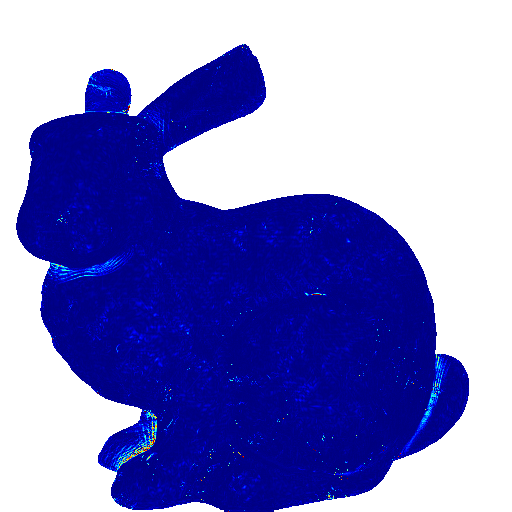}}
			\begin{minipage}{0.02\textwidth} \centering
				\vspace{-5.5em} \makebox[0.5\textwidth]{ $\;\; 15^{\circ}$}\\ \vspace{-0em}
				\makebox[0.5\textwidth]{}\includegraphics[width=0.7\linewidth]{images/color_bar} \\ \vspace{-0.4em}
				\makebox[0.5\textwidth]{ $\;\; 0^{\circ}$}\\
			\end{minipage}\\
			{\includegraphics[ width=\imgsize\textwidth, trim={112px 23px 112px 40px},clip]{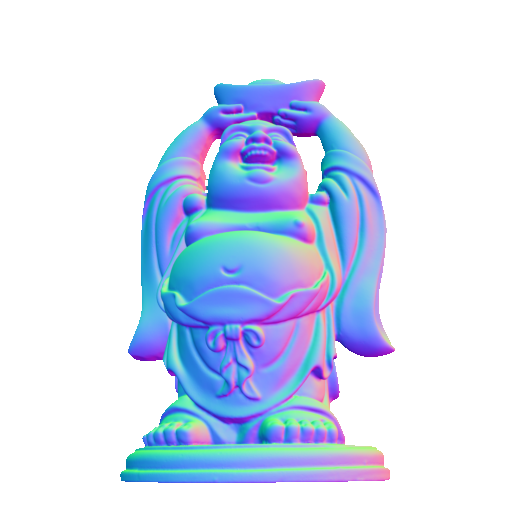}}
			&{\includegraphics[ width=\imgsize\textwidth, trim={112px 23px 112px 40px},clip]{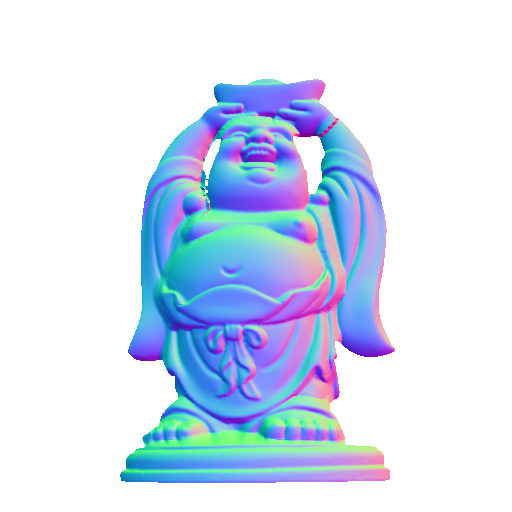}}
			&{\includegraphics[ width=\imgsize\textwidth, trim={112px 23px 112px 40px},clip]{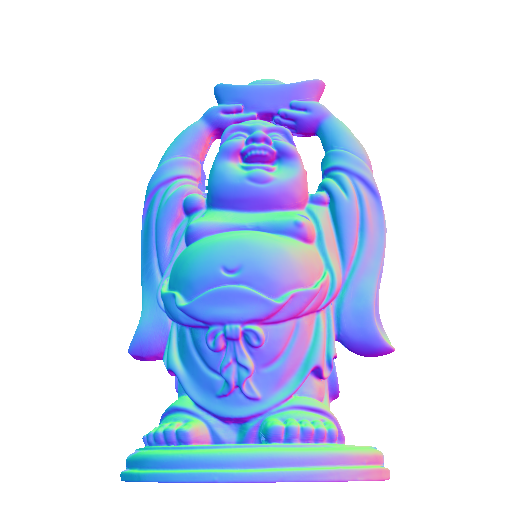}}
			&{\includegraphics[ width=\imgsize\textwidth, trim={112px 23px 112px 40px},clip]{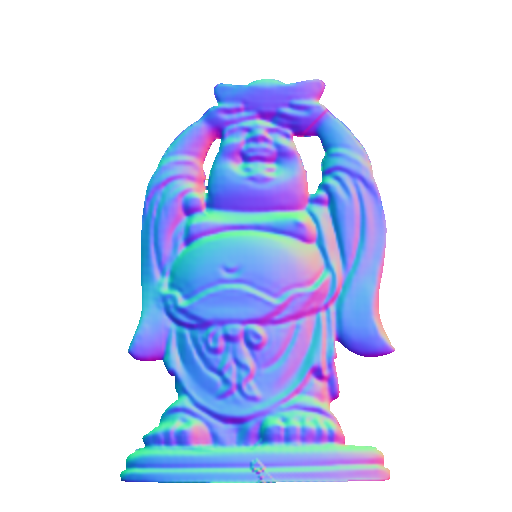}}
			&{\includegraphics[ width=\imgsize\textwidth, trim={112px 23px 112px 40px},clip]{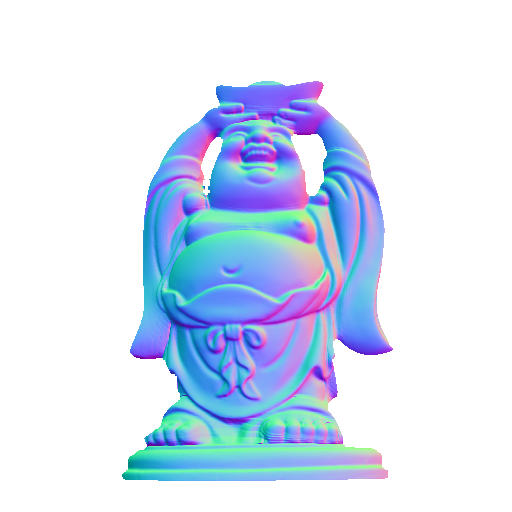}}
			&{\includegraphics[ width=\imgsize\textwidth, trim={112px 23px 112px 40px},clip]{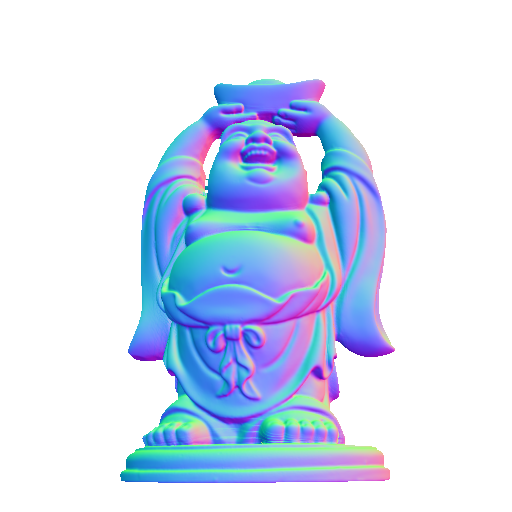}}
			\\
			{\sc Buddha} & 7.84  & 4.44 & 12.19  & 10.44  & 2.11 
			\\
			&{\includegraphics[ width=\imgsize\textwidth, trim={112px 23px 112px 40px},clip]{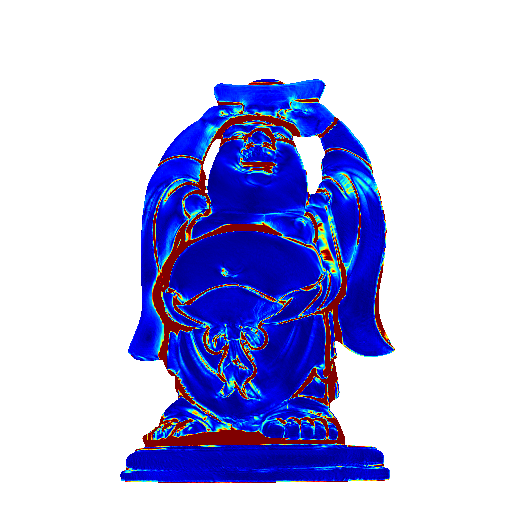}}
			&{\includegraphics[ width=\imgsize\textwidth, trim={112px 23px 112px 40px},clip]{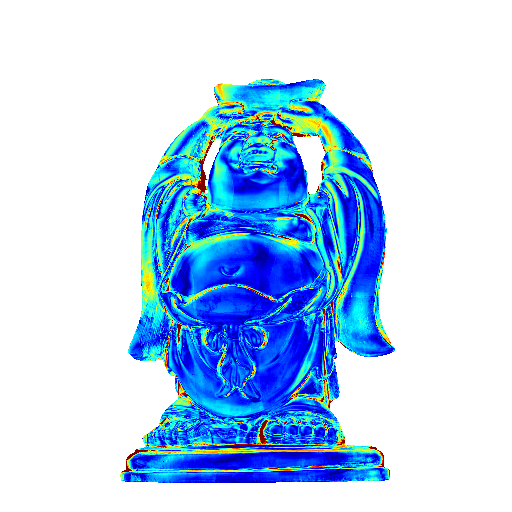}}
			&{\includegraphics[ width=\imgsize\textwidth, trim={112px 23px 112px 40px},clip]{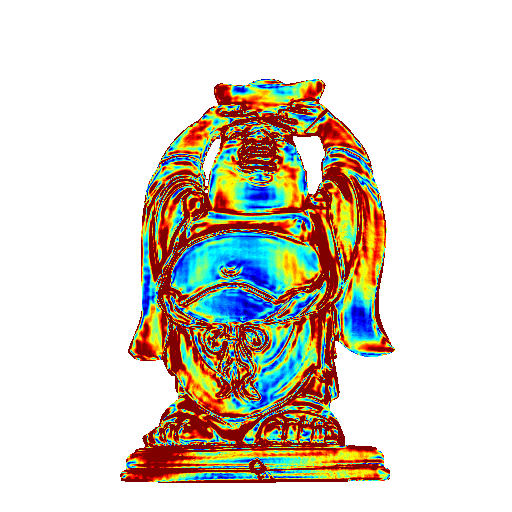}}
			&{\includegraphics[ width=\imgsize\textwidth, trim={112px 23px 112px 40px},clip]{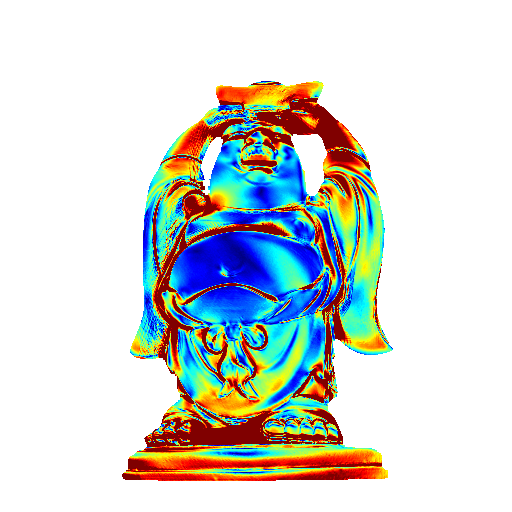}}
			&{\includegraphics[ width=\imgsize\textwidth, trim={112px 23px 112px 40px},clip]{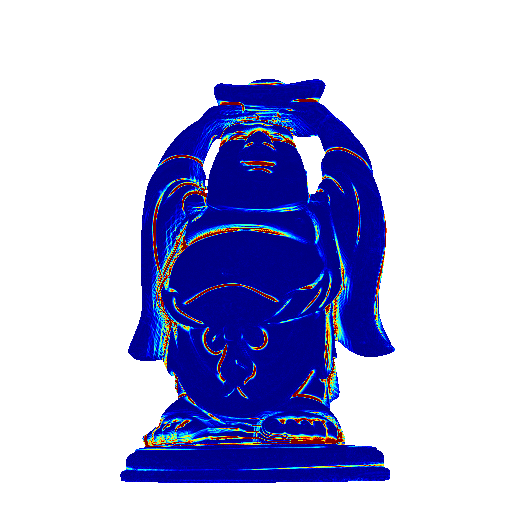}}
			\begin{minipage}{0.02\textwidth} \centering
				\vspace{-7.5em} \makebox[0.5\textwidth]{ $\;\; 15^{\circ}$}\\ \vspace{-0em}
				\makebox[0.5\textwidth]{}\includegraphics[width=0.7\linewidth]{images/color_bar} \\ \vspace{-0.4em}
				\makebox[0.5\textwidth]{ $\;\; 0^{\circ}$}\\
			\end{minipage}\\
		\end{tabular}	
	}
