# Supplementary material for: Edge-preserving Near-light Photometric Stereo with Neural Surfaces
Source: arXiv:2207.04622 source file (2022-07-11)
Supplement: Supplementary file 2 [file supp_synthetic_comp_shape.tex]

\resizebox{1\textwidth}{!}{
		\large
		\begin{tabular}{@{}c:c@{}@{}c@{}@{}c@{}@{}c@{}@{}c@{}}
			GT shape &QD18~\cite{queau2018led}   &LB20~\cite{logothetis2020cnn} & SM20~\cite{santo2020deep}   &MQ16~\cite{mecca2016single} & Ours  \\
			{\includegraphics[ width=\imgsize\textwidth]{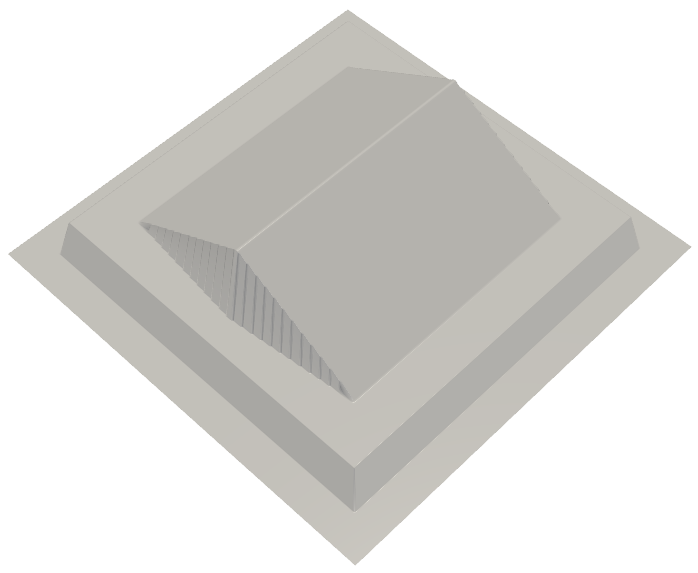}}
			&{\includegraphics[ width=\imgsize\textwidth]{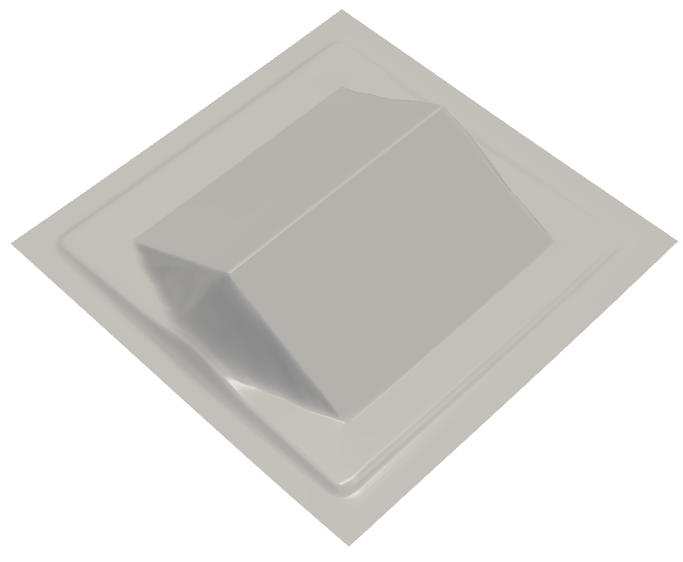}}
			&{\includegraphics[ width=\imgsize\textwidth]{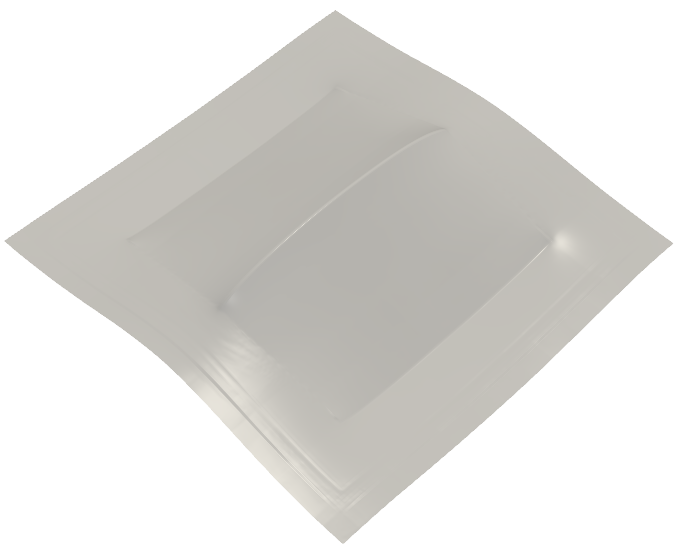}}
			&{\includegraphics[ width=\imgsize\textwidth]{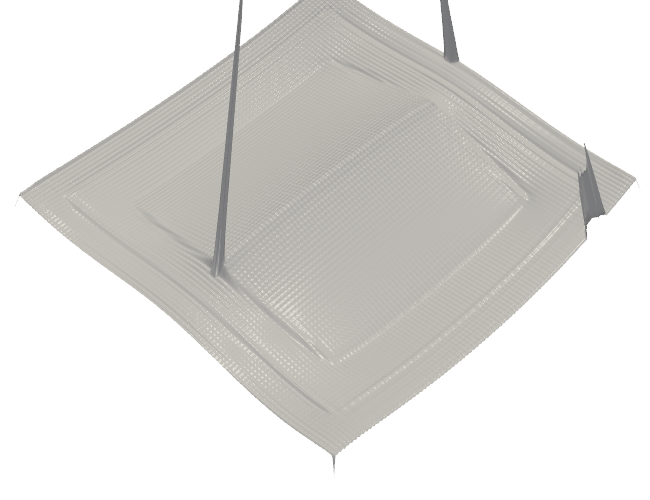}}
			&{\includegraphics[ width=\imgsize\textwidth]{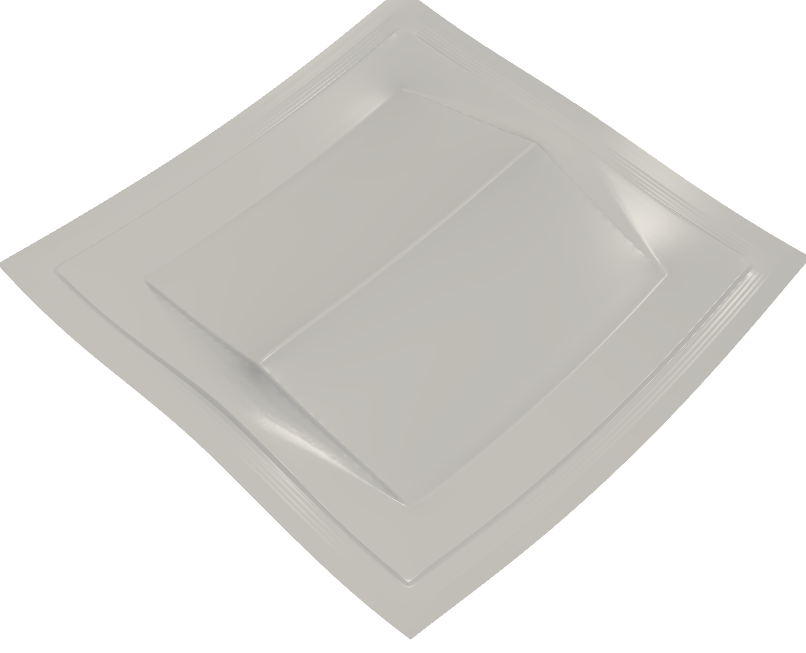}}
			&{\includegraphics[ width=\imgsize\textwidth]{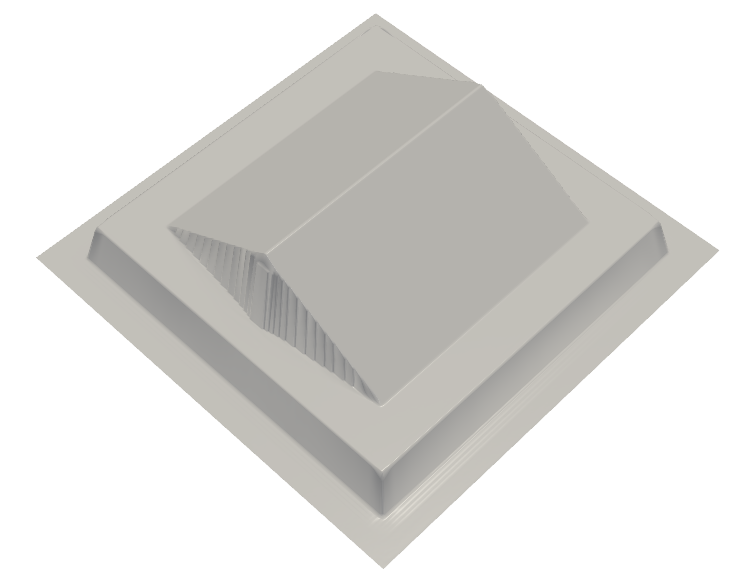}}
			\\
			{\sc Tent} & 0.055  & 0.093   & 0.371 & 0.111  & \textbf{0.003}
			\\
			&{\includegraphics[ width=\imgsize\textwidth, trim={65px 65px 65px 65px},clip]{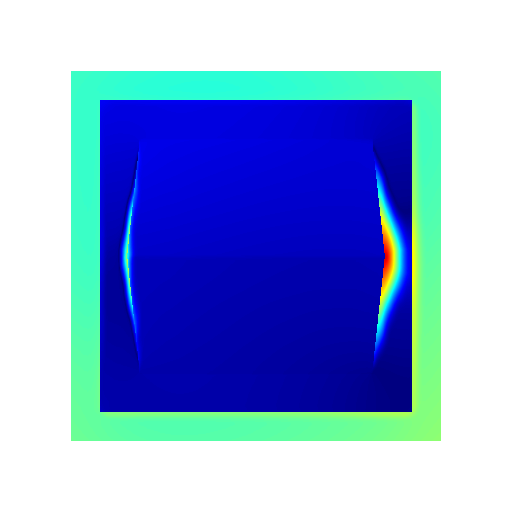}}
			&{\includegraphics[ width=\imgsize\textwidth, trim={65px 65px 65px 65px},clip]{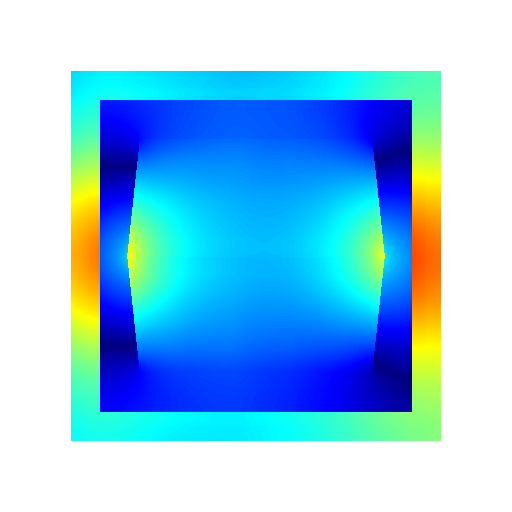}}
			&{\includegraphics[ width=\imgsize\textwidth, trim={65px 65px 65px 65px},clip]{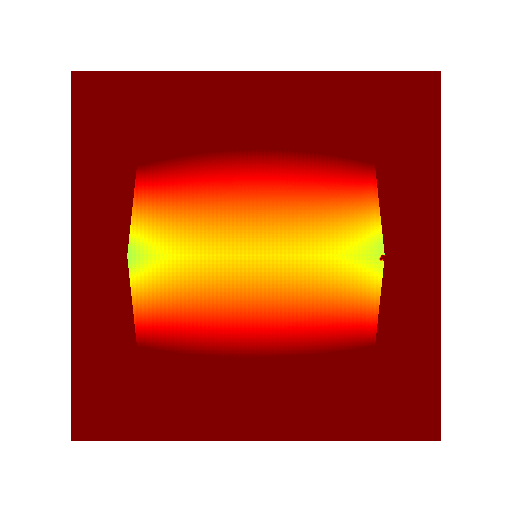}}
			&{\includegraphics[ width=\imgsize\textwidth, trim={65px 65px 65px 65px},clip]{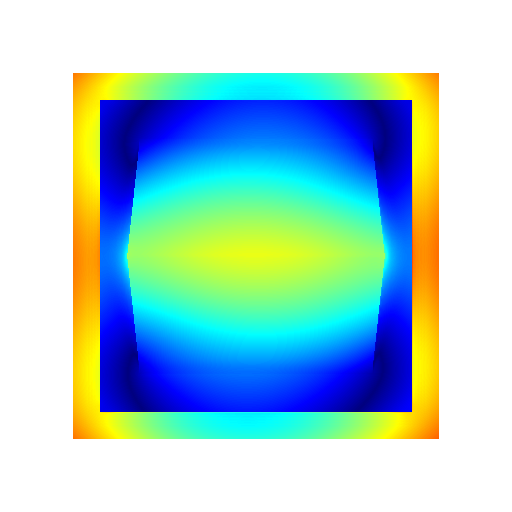}}
			&{\includegraphics[ width=\imgsize\textwidth, trim={65px 65px 65px 65px},clip]{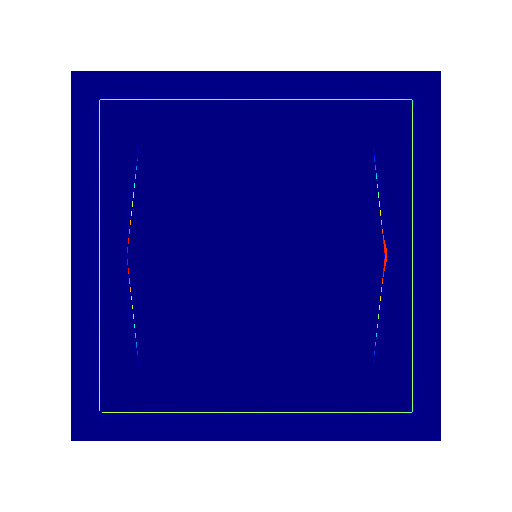}}
			\begin{minipage}{0.02\textwidth} \centering
				\vspace{-5.5em} \makebox[0.5\textwidth]{ $\;\; 0.3\,$m}\\ \vspace{-0em}
				\makebox[0.5\textwidth]{}\includegraphics[width=0.7\linewidth]{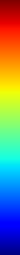} \\ \vspace{-0.4em}
				\makebox[0.5\textwidth]{ $\; 0\;$m}\\
			\end{minipage}\\
			{\includegraphics[ width=\imgsize\textwidth]{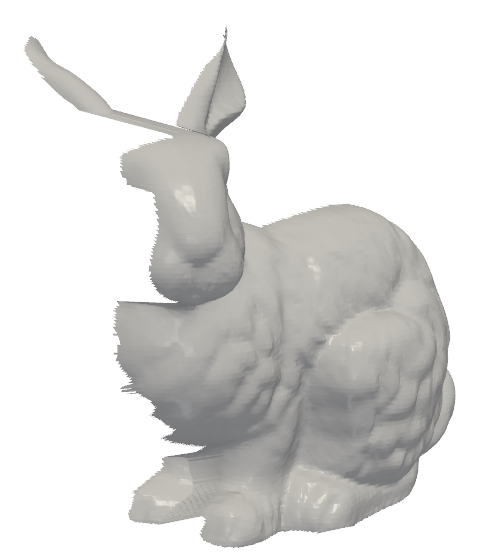}}
			&{\includegraphics[ width=\imgsize\textwidth]{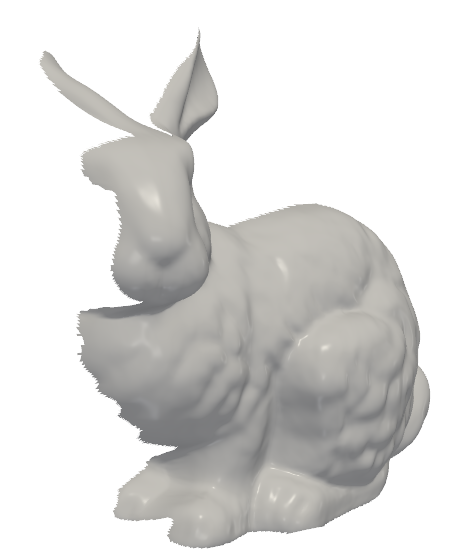}}
			&{\includegraphics[ width=\imgsize\textwidth]{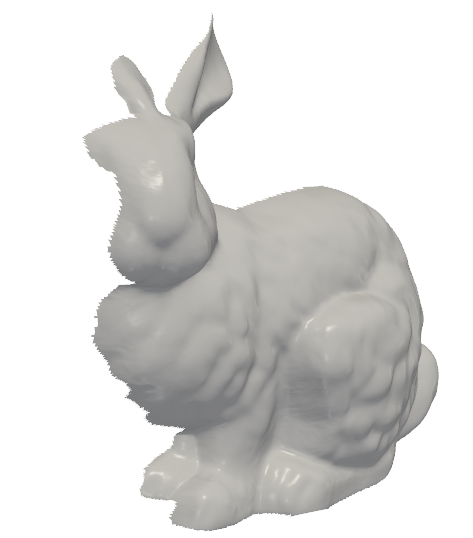}}
			&{\includegraphics[ width=\imgsize\textwidth]{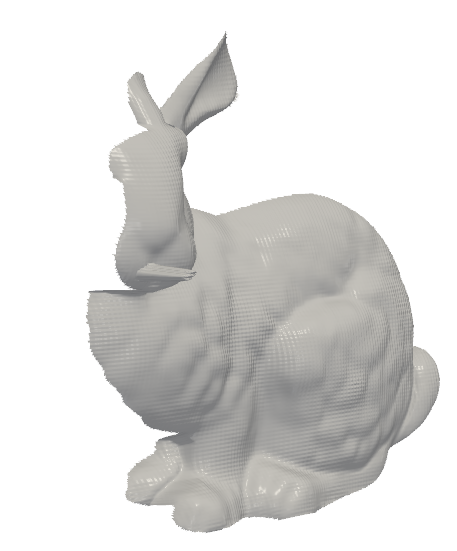}}
			&{\includegraphics[ width=\imgsize\textwidth]{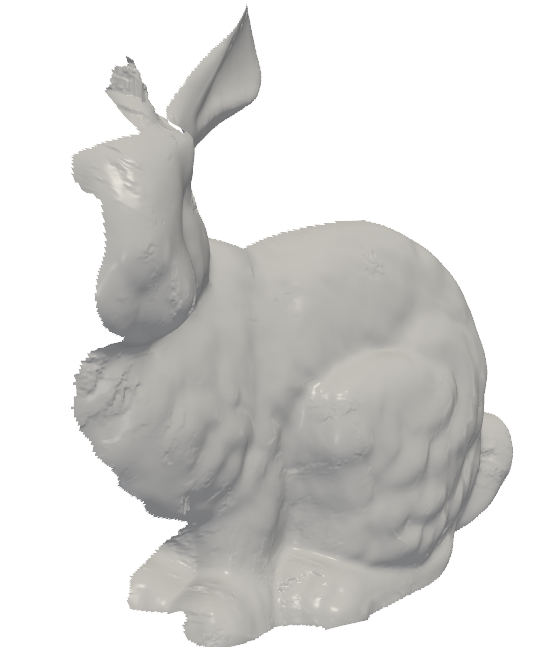}}
			&{\includegraphics[ width=\imgsize\textwidth]{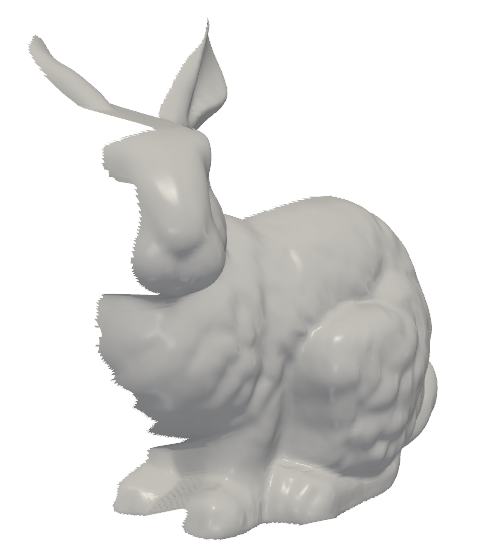}}
			\\
			{\sc Bunny} &  0.024 &  0.031   & 0.058 & 0.060  & \textbf{0.003}
			\\
			&{\includegraphics[ width=\imgsize\textwidth, trim={10px 0px 40px 33px},clip]{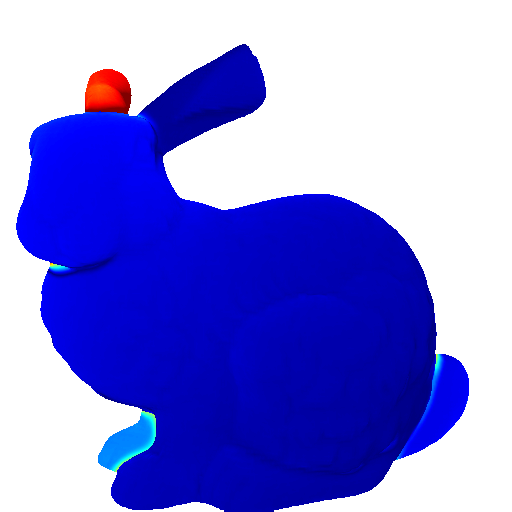}}
			&{\includegraphics[ width=\imgsize\textwidth, trim={10px 0px 40px 33px},clip]{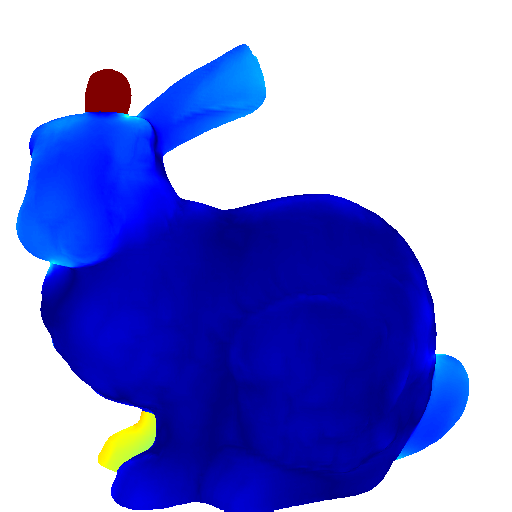}}
			&{\includegraphics[ width=\imgsize\textwidth, trim={10px 0px 40px 33px},clip]{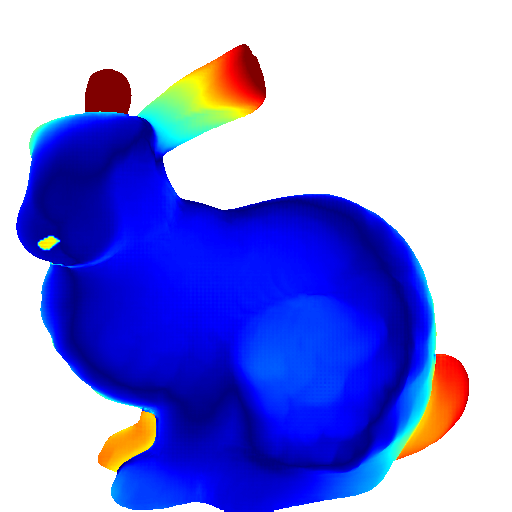}}
			&{\includegraphics[ width=\imgsize\textwidth, trim={10px 0px 40px 33px},clip]{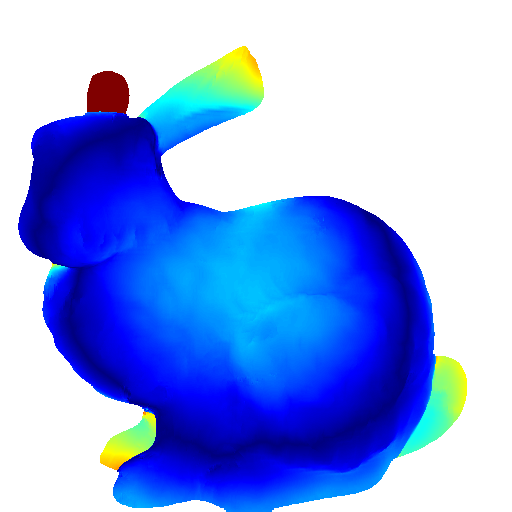}}
			&{\includegraphics[ width=\imgsize\textwidth, trim={10px 0px 40px 33px},clip]{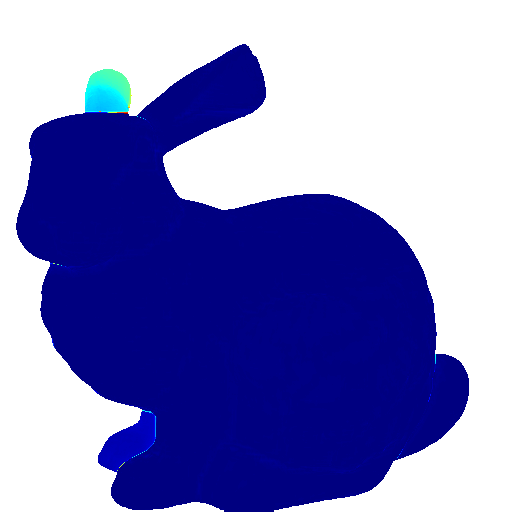}} 
			\begin{minipage}{0.02\textwidth} \centering
				\vspace{-5.5em} \makebox[0.5\textwidth]{ $\;\; 0.3\,$m}\\ \vspace{-0em}
				\makebox[0.5\textwidth]{}\includegraphics[width=0.7\linewidth]{images/color_bar} \\ \vspace{-0.4em}
				\makebox[0.5\textwidth]{ $\; 0\;$m}\\
			\end{minipage}\\
			{\includegraphics[ width=\imgsize\textwidth]{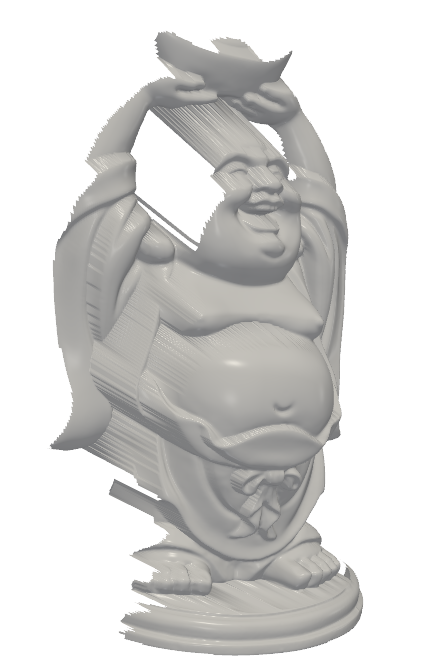}}
			&{\includegraphics[ width=\imgsize\textwidth]{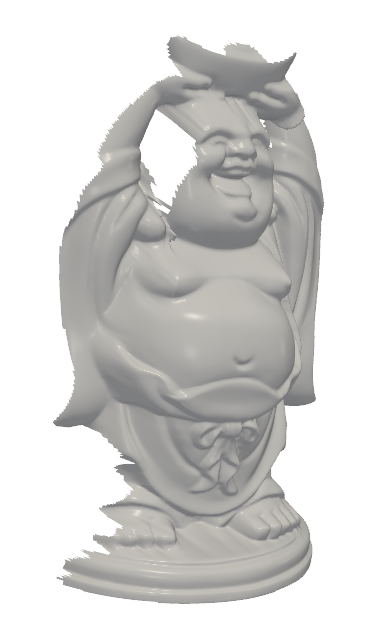}}
			&{\includegraphics[ width=\imgsize\textwidth]{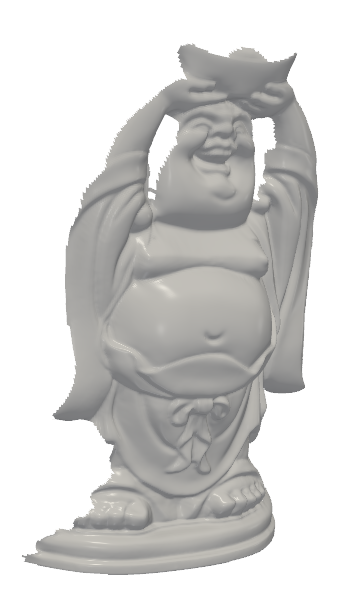}}
			&{\includegraphics[ width=\imgsize\textwidth]{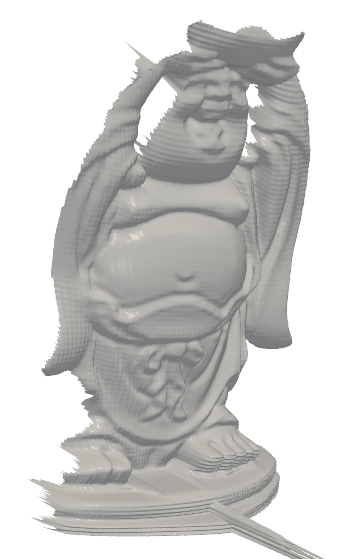}}
			&{\includegraphics[ width=\imgsize\textwidth]{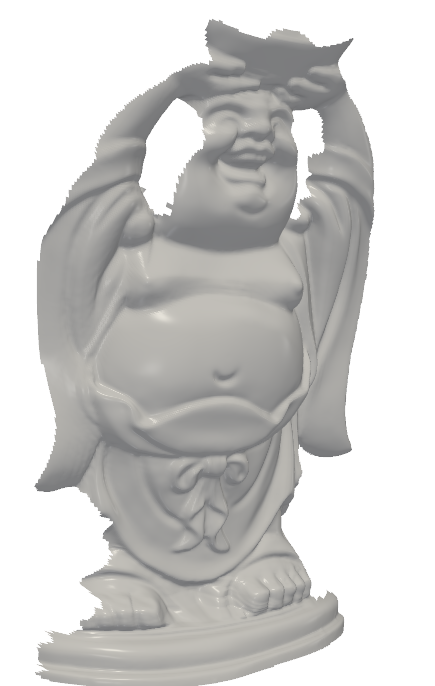}}
			&{\includegraphics[ width=\imgsize\textwidth]{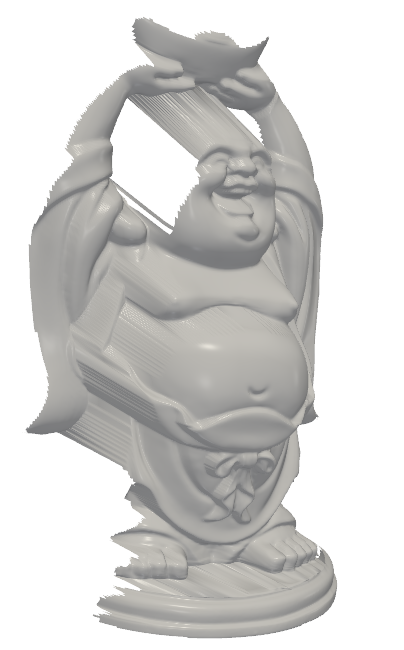}}
			\\
			{\sc Buddha} & 0.071 & 0.129  & 0.149  & 0.097  & \textbf{0.009}
			\\
			&{\includegraphics[ width=\imgsize\textwidth, trim={112px 23px 112px 40px},clip]{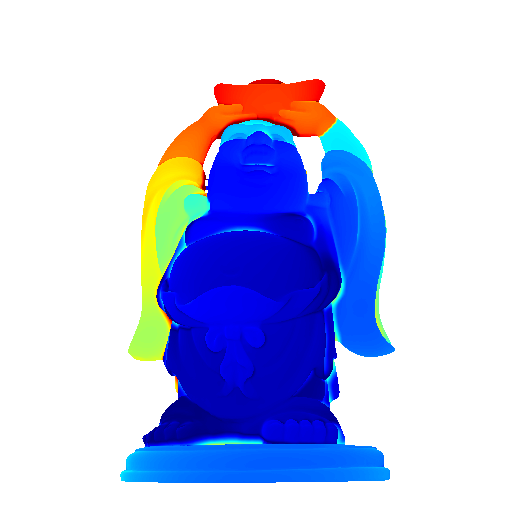}}
			&{\includegraphics[ width=\imgsize\textwidth, trim={112px 23px 112px 40px},clip]{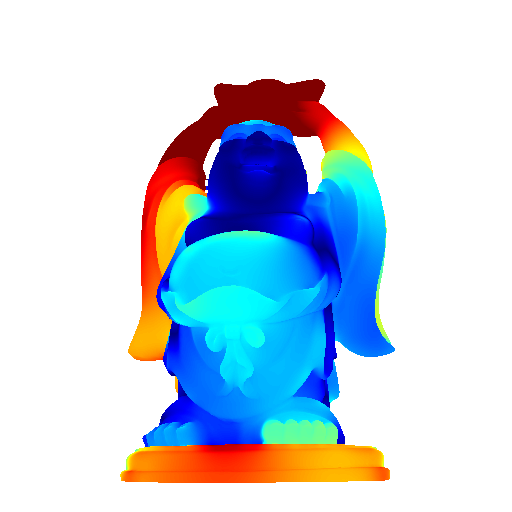}}
			&{\includegraphics[ width=\imgsize\textwidth, trim={112px 23px 112px 40px},clip]{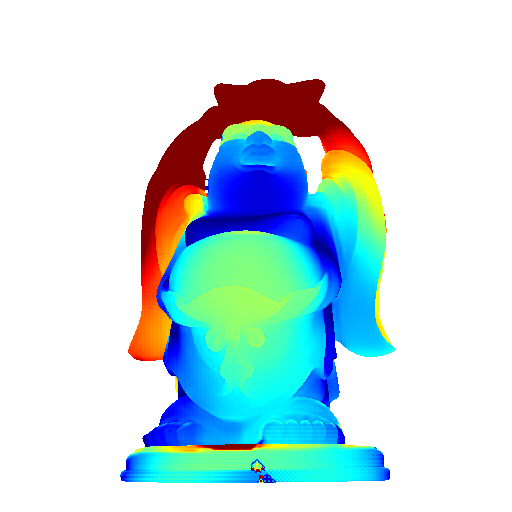}}
			&{\includegraphics[ width=\imgsize\textwidth, trim={112px 23px 112px 40px},clip]{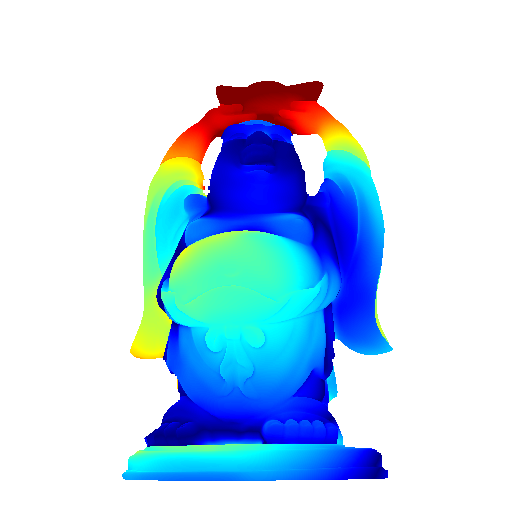}}
			&{\includegraphics[ width=\imgsize\textwidth, trim={112px 23px 112px 40px},clip]{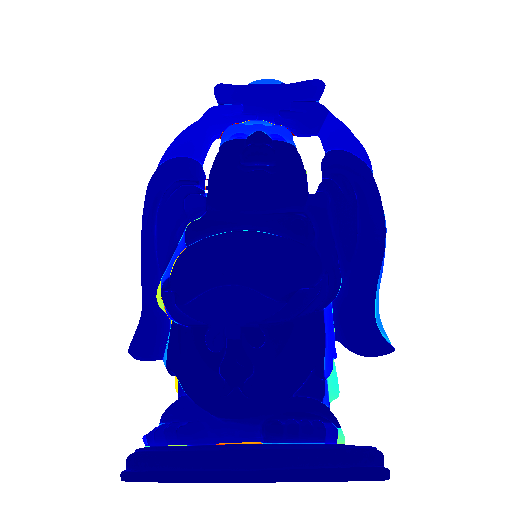}} 
			\begin{minipage}{0.02\textwidth} \centering
				\vspace{-7.5em} \makebox[0.5\textwidth]{ $\;\; 0.3\,$m}\\ \vspace{-0em}
				\makebox[0.5\textwidth]{}\includegraphics[width=0.7\linewidth]{images/color_bar} \\ \vspace{-0.4em}
				\makebox[0.5\textwidth]{ $\; 0\;$m}\\
			\end{minipage}\\
		\end{tabular}	
	}
